# Supplementary material for: Metrics-in-the-Loop: Complexity Feedback Reshapes Agent-Written Code
Source: arXiv:2611.23817 source file (2026-11-18)
Supplement: Supplementary file 1 [file tracestyle.tex]

\makeatletter
\newcommand{\trfontsans}{\@ifundefined{T1/cmr/m/n/10}{\sffamily}{\fontencoding{T1}\fontfamily{IBMPlexSans-TLF}\selectfont}}
\newcommand{\trfontmono}{\@ifundefined{T1/cmr/m/n/10}{\ttfamily}{\fontencoding{T1}\fontfamily{IBMPlexMono-TLF}\selectfont}}
\newcommand{\trmedium}{\@ifundefined{T1/cmr/m/n/10}{\bfseries}{\fontseries{medium}\selectfont}}
\newcommand{\tr@verbfont}{\normalfont\trfontmono}
\begingroup\lccode`\~=`\'\lowercase{\endgroup\def\tr@sq{\def~{\textquotesingle}}}
\begingroup\lccode`\~=`\`\lowercase{\endgroup\def\tr@bq{\def~{\textasciigrave}}}
\def\tr@upquote{\expandafter\def\expandafter\@noligs\expandafter{\@noligs\tr@sq\tr@bq}}
\makeatother
\definecolor{trInk}{HTML}{2B2926}\definecolor{trMuted}{HTML}{6B665C}\definecolor{trSand}{HTML}{F6F3EC}\definecolor{trGrid}{HTML}{E2DCCF}
\definecolor{trFeedback}{HTML}{C8623D}\definecolor{trFeedbackBg}{HTML}{F9EFE9}
\definecolor{trAgent}{HTML}{2F6EA3}\definecolor{trAgentBg}{HTML}{EEF3F8}
\definecolor{trAfter}{HTML}{5E7F48}\definecolor{trAfterBg}{HTML}{F0F4EA}
\definecolor{trBefore}{HTML}{8A8478}\definecolor{trBeforeBg}{HTML}{F6F3EC}
\definecolor{trResultBg}{HTML}{FFFFFF}
\definecolor{trKey}{HTML}{2B2926}\definecolor{trKeyBg}{HTML}{F6F3EC}\definecolor{trOver}{HTML}{A8482A}\definecolor{trOk}{HTML}{4E6B3A}
\makeatletter
\tcbset{trbase/.style={enhanced, arc=1.6mm, boxrule=0.5pt, left=4pt, right=4pt, top=1.5pt, bottom=1.5pt,
  toptitle=1.4pt, bottomtitle=0pt, titlerule=0pt, fonttitle=\trfontsans\trmedium\scriptsize,
  fontupper=\trfontsans\scriptsize, before upper={\let\verbatim@font\tr@verbfont\tr@upquote},
  before skip=2.5pt, after skip=2.5pt}}
\makeatother
\tcbset{trlabel/.style={colframe=#1, colback=#1Bg, colbacktitle=#1Bg, coltitle=#1}}
\newtcolorbox{trFeedbackBox}[1]{trbase, trlabel=trFeedback, title={SlapKit feedback\hfill{\color{trMuted}#1}}}
\newtcolorbox{trAgentBox}[1]{trbase, trlabel=trAgent, title={agent\hfill{\color{trMuted}#1}}}
\newtcolorbox{trResultBox}{trbase, arc=1.2mm, boxrule=0.4pt, colback=trResultBg, colframe=trBefore!55,
  left=3pt, top=0.5pt, bottom=0.5pt, before skip=1pt, after skip=2pt}
\newtcolorbox{trBeforeBox}[1]{trbase, trlabel=trBefore, fontupper=\trfontsans\tiny,
  title={code before\hfill{\color{trMuted}#1}}}
\newtcolorbox{trAfterBox}[1]{trbase, trlabel=trAfter, fontupper=\trfontsans\tiny,
  title={code after\hfill{\color{trMuted}#1}}}
\newtcolorbox{trMeasuredBox}{trbase, colback=white, colframe=trBefore!70, boxrule=0.4pt, fontupper=\small}
\newcommand{\trChip}[2]{\tcbox[enhanced, on line, arc=1.2mm, boxrule=0.4pt, colback=#1Bg, colframe=#1,
  left=2.5pt, right=2.5pt, top=0.2pt, bottom=0.2pt, fontupper=\trfontsans\scriptsize\color{#1!85!black}]{#2}}
\newcommand{\trLegend}{\noindent\trChip{trFeedback}{SlapKit feedback}\ \trChip{trAgent}{agent tool call}\
  \tcbox[enhanced, on line, arc=1.2mm, boxrule=0.4pt, colback=white, colframe=trBefore!55, left=2.5pt, right=2.5pt,
  top=0.2pt, bottom=0.2pt, fontupper=\trfontsans\scriptsize\color{trMuted}]{tool result}\ \trChip{trBefore}{code before}\
  \trChip{trAfter}{code after}\par}
\newcommand{\trNote}[1]{{\trfontsans\scriptsize\itshape\color{trAgent!85!black}#1}\par}
\newcommand{\trFoot}[1]{\par\vspace{1pt}{\trfontsans\scriptsize\color{trAfter!80!black}#1}\par}
\newtcolorbox{trTakeawayBox}{trbase, colback=white, colframe=trInk!80, colbacktitle=white, coltitle=trInk,
  boxrule=0.5pt, fontupper=\small, title={Takeaway}}
\newtcolorbox{trTableBox}[1]{trbase, colback=white, colframe=trBefore!80, colbacktitle=white, coltitle=trInk,
  fontupper=\scriptsize, title={measured complexity\hfill{\color{trMuted}#1}}}
\newcommand{\trOverL}{\textcolor{trOver}{\textbf{over}}}
\newcommand{\trOkL}{\textcolor{trOk}{\textbf{within}}}
\newcommand{\trSrc}[1]{\par\vspace{1pt}{\trfontsans\tiny\color{trMuted}Where to check: #1}\par}
\newcommand{\trRecommended}{\noindent\tcbox[enhanced, on line, arc=1.2mm, boxrule=0.5pt, colback=trAfterBg,
  colframe=trAfter, left=3pt, right=3pt, top=0.4pt, bottom=0.4pt,
  fontupper=\trfontsans\trmedium\scriptsize\color{trAfter!85!black}]{recommended for the final appendix}\par\vspace{2pt}}
\newtcolorbox{trPromptBox}[2][]{trbase, breakable, trlabel=trBefore, title={#2}, #1}
